# Supplementary material for: Image Representations Learned With Unsupervised Pre-Training Contain Human-like Biases
Source: arXiv:2010.15052 source file (2021-01-27)
Supplement: Supplementary file 1 [file supplemental.tex]

\documentclass[sigconf,table]{acmart} %
\settopmatter{printacmref=false} %

\renewcommand\footnotetextcopyrightpermission[1]{} %

\AtBeginDocument{%
  \providecommand\BibTeX{{%
    \normalfont B\kern-0.5em{\scshape i\kern-0.25em b}\kern-0.8em\TeX}}}

\input{tex/meta}
\arxivfalse %
\blindfalse
\draftfalse

\begin{document}

\title[\stitle]{\textit{Supplementary Material for}\\\ttitle}

\author{Ryan Steed}
\email{ryansteed@cmu.edu}
\affiliation{%
  \institution{Carnegie Mellon University}
  \city{Pittsburgh}
  \state{Pennsylvania}
  \country{USA}
}

\author{Aylin Caliskan}
\email{aylin@gwu.edu}
\affiliation{%
  \institution{George Washington University}
  \city{Washington}
  \state{District of Columbia}
  \country{USA}
}

\maketitle

\input{tex/appendix}

\clearpage

\bibliographystyle{ACM-Reference-Format}
\bibliography{references}

\end{document}
